# Supplementary material for: Globally Governed Session Semantics
Source: arXiv:1412.5943 source file (2015-03-01)
Supplement: Supplementary file 2 [file app-typingrule.tex]

\section{Appendix for Typing Rules}
\label{app:typing}
\subsection{Two projections}
\label{subsec:projection}
The relation between global and local types is formalised by 
the standard projection function \cite{HYC08}.
\begin{definition}[Global projection and projection set]
\label{def:projection}
\rm
The projection of a global type $G$ 
onto a participant $\p$ is defined by induction on $G$:
\[
\small
\begin{array}{ll}
\begin{array}{ll}
\proj{\valuegt{\p'}{\q}{\U} \G}{\p}\\ 
\quad = \left\{
	\begin{array}{lcl}
		\tout{\q}{\U} \proj{\G}{\p} & \quad & \p = \p'\\
		\tinp{\p'}{\U} \proj{\G}{\p} & \quad & \p = \q \\
		\proj{\G}{\p} & \quad & \textinmath{otherwise}
	\end{array} \right. 
\end{array}
&
\begin{array}{ll}
\proj{\selgtG{\p'}{\q}}{\p}\\ 
\quad = \left\{
	\begin{array}{lcl}
	\tsels{\q}{\set{l_i:\proj{\G_i}{\p}}_{i \in I}} & \quad & \p = \p'\\
	\tbras{\p'}{\set{l_i:\proj{\G_i}{\p}}_{i \in I}} & \quad & \p = \q \\
	\proj{\G_1}{\p} & \quad & \text{if}\  \forall j\in I.\
              \proj{\G_1}{\p}=\proj{\G_j}{\p}
	\end{array} \right.\\
\end{array}
\\
\begin{array}{ll}
	\proj{(\recgt{t}{\G})}{\p} = 
\left\{
	\begin{array}{lcl}
		\trec{t}{(\proj{\G}{\p})} & \quad & \p \in G\\
                \tinact                   & \quad & \textinmath{otherwise}
	\end{array} \right.\\
\end{array}
&
\begin{array}{l}
	\proj{\vargt{t}}{\p} = \tvar{t} \quad 
	\proj{\inactgt}{\p} = \tinact 
\end{array}
\end{array}
\]
Then the {\em projection set} of $\typed{s} \G$
is defined as 
$\projset{\typed{s} \G} =
\set{\typedrole{\s}{\p} \proj{\G}{\p}\setbar \p \in \roles{\G}}$
where 
$\roles{\G}$ denotes the set of the roles appearing in $\G$. 
\end{definition}
%Inactive $\inactgt$ and recursive variable $\vargt{t}$ types
%are projected to their respective local types.
%We project a global type $\valuegt{\p'}{\q}{\U} \G$ to
%party $\p$ as a sending local type if $\p = \p'$ and as
%a receiving local type if $\p = \q$. In any case the
%continuation of the projection is $\proj{\G}{\p}$.
%For $\selgtG{\p}{\q}$ global type the projection is the 
%select local type for $\p = \p'$ and the branch local type  $\p = \q$.
%Otherwise we use the projection of one of the of one of the
%$\set{\G_i \setbar i \in I}$ global types (all types $\G_i$
%should have the same projection with respect to $\p$).
%Recursion $\recgt{t}{\G}$ is projected  onto a local type using local
%recursion and the projection of the global type $\G$ with
%respect to $\p$. 

We also need the following projection from a local type $\T$ 
to produce binary session types for defining the equivalence
relations later. 

\begin{definition}[Local projection]\rm
\label{def:localprojection}
The projection of a local type $T$ 
onto a participant $\p$ is defined by induction on $T$:
\[
\small
	\begin{array}{rclrcl}
		\proj{\tout{\p}{\U} T}{\q} & = & \left\{
		\begin{array}{lcl}
			\btout{\U} \proj{\T}{\q} & \quad & \textrm{\q = \p}\\
			\proj{\T}{\q} & \quad & \textrm{otherwise} 
		\end{array}
		\right.\quad 

		\proj{\tinp{\p}{\U} T}{\q} & = & \left\{
		\begin{array}{lcl}
		\btinp{\U} \proj{\T}{\q} & \quad & \textrm{\q = \p}\\
			\proj{\T}{\q} & \quad & \textrm{otherwise}
		\end{array}
		\right.
\end{array}
\]
\[
\begin{array}{rcl}
		\proj{\tsel{\p}{l_i: T_i}_{i \in I}}{\q} & = & \left\{
		\begin{array}{lcl}
			\btsel{l_i:\proj{\T_i}{\q}}_{i \in I} & \quad & \textrm{\q = \p}\\
			\proj{\T_1}{\q} & \quad & 
\text{if} \ \forall i\in I. \proj{\T_i}{\q} = \proj{\T_1}{\q}
		\end{array}
		\right.\\

		\proj{\tbra{\p}{l_i: T_i}_{i \in I}}{\q} & = & \left\{
		\begin{array}{lcl}
			\btbra{l_i:\proj{\T_i}{\q}}_{i \in I} & \quad & \textrm{\q = \p}\\
			\proj{\T_1}{\q} & \quad & 
\text{if} \ \forall i\in I. \proj{\T_i}{\q} = \proj{\T_1}{\q}
		\end{array}
		\right.\\

%		\proj{(\trec{t}{\T})}{\q} & = & \trec{t}{(\proj\T\q)}\\
%		\proj{\vart{t}}{\q} & = & \vart{t}\\
%		\proj\tinact\q & = & \tinact
	\end{array}
\]
The rest is similar as Definition \ref{def:projection}. 
\end{definition}
The duality over the projected types are defined as: 
$\tinact  =  \dual{\tinact}$, $\vart{t}  = \dual{\vart{t}}$,  
$\dual{\trec{t}{T}} = \trec{t}{\dual{T}}$, 
$\dual{\btout{U} T} = \btinp{U} \dual{T}$, 
$\dual{\btinp{U} T} = \btout{U} \dual{T}$, 
$\dual{\btsel{l_i:T_i}_{i \in I}} = \btbra{l_i:\dual{T_i}}_{i \in I}$
and  
$\dual{\btbra{l_i:T_i}_{i \in I}} = \btsel{l_i:\dual{T_i}}_{i \in I}$.  
We note that if $\p, \q \in \roles{G}$ then
$\proj{(\proj{\G}{\p})}{\q} =
       \dual{\proj{(\proj{\G}{\q})}{\p}}$. 

%Inactive local type and the recursive variable are always projected
%to their corresponding binary session types syntax. Recursion
%operator $\trec{t}{\T}$ is projected onto the corresponding 
%binary session types syntax.
%$\tout{\p}{\U} T, \tinp{\p}{\U} T$ are projected with respect to $\q$
%to binary session type send and binary session type receive respectively, 
%and continue with the projection of $T$ on $q$ if $\p = \q$. 
%If $\p \not= \q$ local projection continues with the projection of $T$.
%Similar argument for $\tsel{\p}{l_i: T_i}_{i \in I}, \tbra{\p}{l_i: T_i}_{i \in I}$,
%where in the case of $\p = \q$ the projection follows binary session types.
%In the case where $\p \not= \q$ we project one of the continuations in
%$\set{T_i}_{i \in I}$ since we expect all the projections to be the same.

%We define the session duality relation on local projections.
%\begin{definition}[Duality]
%\[
%	\begin{array}{rclcrclcrclcrclcrcl}
%		\tinact & = & \dual{\tinact} &\quad& \vart{t} & = & \dual{\vart{t}} &\quad& 
%		\dual{\trec{t}{T}} = \trec{t}{\dual{T}} & \quad &
%		\dual{\btout{U} T} &=& \btinp{U} \dual{T} & \quad
%		\dual{\btinp{U} T} &=& \btout{U} \dual{T}
%	\end{array}
%\]
%\[
%	\begin{array}{rclcrclcrclcrclcrcl}
%		\dual{\btsel{l_i:T_i}_{i \in I}} & = & \btbra{l_i:\dual{T_i}}_{i \in I} &\quad& 
%		\dual{\btbra{l_i:T_i}_{i \in I}} & = & \btsel{l_i:\dual{T_i}}_{i \in I}
%	\end{array}
%\]
%\end{definition}

%\input{figures/fig-types}

\subsection{Typing system and its properties}
\label{subsec:typing}
The typing judgements for expressions and processes are of the shapes:
\begin{eqnarray*}
	\Gproves{\e}{\So} \quad \textinmath{ and } \quad \Gtprocess{\PP}{\De}
\end{eqnarray*}
where $\Gamma$ is the standard environment 
which associates variables to sort types, shared names to
global types and process variables to session environments; and 
$\Delta$ is the session environment which associates channels to session types.
Formally we define: 
\begin{eqnarray*}
	\Ga \bnfis \es \bnfbar \Gacat{\typed{u} \So} \bnfbar
        \Gacat{\typed{\varp{X}} \De}\quad \textinmath{ and } \quad \De \bnfis \es \bnfbar \Decat{\typedrole{s}{\p} \T}
\end{eqnarray*}
assuming we can write $\Gacat{\typed{u} \So}$ if $u\not\in\dom{\Gamma}$. 
We extend this to a concatenation for typing environments as 
$\De \cat \De'=  \De \cup \De'$.
We define coherency of session environments as follows:
%We use the following definitions for coherency of session 
%session environments.  

\begin{definition}[Coherency]\rm 
\label{def:coherency}
Typing $\De$ is {\em coherent 
	with respect to session $s$}
	(notation $\cohses{\De}{s}$) if
	$\forall \srole{s}{\p}: T_\p, \srole{s}{\q}: T_\q \in \De$ with $\p \not= \q$
	then
	$\proj{T_\p}{\q} = \dual{\proj{T_\q}{\p}}$.
	A typing $\De$ is {\em coherent}
	(notation $\coherent{\De}$) if 
	it is coherent with respect to all $s$ in its domain.
	We say that the typing judgement $\Gtprocess{\PP}{\De}$ 
	is {\em coherent} if $\coherent{\De}$. 
\end{definition}

The typing rules are essentially identical to the communication
typing system for programs 
in \cite{BettiniCDLDY08} (since~we do not require
queues). %We leave the rules in Figure \ref{fig:synch-typing} 
%in Appendix \ref{app:typing}. 
%The rest of the paper can be read without knowing the 
%typing system. 

We say a typing $\De$ is {\em fully coherent}
		(notation $\fcoherent{\De}$) if
		it is coherent and
		if $\srole{s}{\p}:T_\p \in \De$ then
                for all	$\q \in \roles{T_\p}$, 
		$\srole{s}{\q} : T_\q \in \De$.

\input{figures/fig-typing}

Figure \ref{fig:synch-typing} defines the typing system.
Rule $\trule{Name}$ types a shared name or
shared variable to type $S$.
Boolean $\true, \false$ are typed with the $\bool$ 
type via rule $\trule{Bool}$.
Logical expressions are also typed with the $\bool$
type via rule $\trule{And}$, etc.
Rules $\trule{MReq}$ and $\trule{MAcc}$ check that the local type of
a session endpoint agrees with the global type of the initiating shared name.
Rules $\trule{Send}$ and $\trule{Recv}$ prefix the local type with
send and receive local types, respectively after checking
the type environment for the sending value type (receiving variable type resp.).
Delegation is typed under rules $\trule{Deleg}$ and $\trule{Srecv}$
where we check type consistency of the delegating/receiving session endpoint.
%to have
%consistent local type with the delegating/receiving session role. 
Rules $\trule{Sel}$ and $\trule{Bra}$ type select and 
branch processes, respectively.  A select process uses the select
local type. A branching process checks that all continuing process
have a consistent typing environments. $\trule{Conc}$ types a parallel
composition of processes by checking the disjointness of their
typing environments. Conditional is typed with 
$\trule{If}$, where we check the expression $\e$ to be of $\bool$ 
type and the branching processes to have the same typing environment.
Rule $\trule{Nres}$
defines the typing for shared name restriction. Rule $\trule{Sres}$
uses the full coherency property to restrict a session name. 
Recursive rules 
$\trule{Var}$ and $\trule{Rec}$ are standard. Finally the inactive
process $\inact$ is typed with the complete typing  environment, where
every session endpoint is mapped to the inactive local type $\tinact$.
The following
theorem is proved in 
\cite{BettiniCDLDY08}.   

\begin{theorem}[Subject reduction]
\label{the:subject}
If $\Gtprocess{P}{\De}$ is coherent and $P \Red P'$ then
	$\Gtprocess{P'}{\De'}$ is coherent with $\De \typingRed \De'$ .
\end{theorem}
