# Supplementary material for: Globally Governed Session Semantics
Source: arXiv:1412.5943 source file (2015-03-01)
Supplement: Supplementary file 3 [file org-completeness-proof.tex]

\subsection{Proof for Lemma \ref{lem:bis-cong} (2)}
\label{app:bis-complete}

%\begin{proof}

	We rely on the fact that bisimulation has a stratifying
	definition.

	\begin{itemize}
		\item	$({\govwbs})_0$ is the union of all configuration relations,
			$\tprocess{E, \Ga}{P}{\De_1}\ R\ Q \hastype{\De_2}$.
		\item	$\tprocess{E, \Ga}{P}{\De_1} ({\govwbs})_n Q \hastype{\De_2}$ if 
		\begin{itemize}
			\item	$\tprocess{E, \Ga}{P}{\De_1} \trans{\ell} \tprocess{E', \Ga}{P'}{\De_1'}$ then
				$\tprocess{E, \Ga}{Q}{\De_2} \Trans{\ell} \tprocess{E', \Ga}{Q}{\De_2'}$ and
				$\tprocess{E', \Ga}{P'}{\De_1'} ({\govwbs})_{n-1} Q' \hastype{\De_2'}$
			\item The symmetric case.
		\end{itemize}
		\item $({\govwbs})_n = \bigcap_{0 \leq i \leq n} 
({\govwbs})_i$ 
	\end{itemize}

	From coinduction theory, we know that $(\bigcap_{\forall n} ({\govwbs})_n) = \govwbs$.

	%We need to prove that if $\tprocess{E, \Ga}{P}{\De_1} \govcongs Q \hastype{\De_2}$ then $\tprocess{E, \Ga}{P}{\De_1} {\govwbs}_n Q \hastype{\De_2}, \forall n$.

Note that by Lemma \ref{lemma:Bisimulation_typing_relation}, 
if $\tprocess{E, \Ga}{\PP_1}{\De_1}\ \govwbs\ \noGtprocess{\PP_2}{\De_2} $, then $\De_1 \bistyp \De_2$. Notice also that 
in Definition \ref{def:grc}(2), the definition implies  
$\De_1 \typingred^\ast \De'_1$ and 
$\De_2 \typingred^\ast \De'_2$ by 
Theorem~\ref{the:subject}.

We proceed by defining a processes $T\lrangle{N, \vec{\ell_n}}$ called tests.
A test process is composed in parallel with a process and is able to interact 
with a sequence of actions that the latter process may produce.

Below we state the steps we take for the proof:
\[
	\begin{array}{lll}
		1.	\textrm{If } 	& \tprocess{E, \Ga}{P_1}{\De_1} \govcongs P_2 \hastype{\De_2} \ \ \textrm{ implies} \\
		2. 			& \tprocess{E, \Ga}{P_1 \Par T\lrangle{N, \vec{\ell_n}}}{\De_1} \govcongs
					P_2 \Par T\lrangle{N, \vec{\ell_n}} \hastype{\De_2} \ \ \textrm{ then} \\
		3.	 \forall n,	& \tprocess{E, \Ga}{P_1}{\De_1} ({\govwbs})_n P_2 \hastype{\De_2} \ \ \textrm{ implies} \\
					& \tprocess{E, \Ga}{P_1}{\De_1} {\govwbs} P_2 \hastype{\De_2}
	\end{array}
\]

	The first step is trivial from the definition of reduction closed congruence $\govcongs$.
	From the first step we need to do a case analysis on the test process $T\lrangle{N, \vec{\ell_n}}$
	for the second step. Finally standard induction gives us the result of the second step.

	We give the definition for $T\lrangle{N, \vec{\ell_n}}$:

	$T\lrangle{N, succ, \vec{\ell_n}} = \Pi_{i \in I}Q\lrangle{N, n, \vec{\ell_i}}$

	\noi where
	\begin{enumerate}
		\item $i \in I$
		\item $\bigcup_{i \in I} \vec{\ell_i} = \vec{\ell_n}$
		\item $n \bnfis \srole{s}{\p} \bnfbar a$ 
		\item $N \bnfis \es \bnfbar N \cat \srole{s}{\p} \bnfbar N \cat a$
		is a set of names for testing the receiving objects, and
		\item $succ$ is a fresh name
	\end{enumerate}

	\noi to define
	\begin{enumerate}
		\item	$
				\begin{array}{lcl}
					Q\lrangle{N, a, \actacc{a}{A}{s} \cat \vec{\ell_i}} & = & 
					\req{a}{n}{x} Q\lrangle{N, \srole{s}{n}, \vec{\ell_{j}}} \Par \dots
					\acc{a}{\p_1}{x} Q\lrangle{N, \srole{s}{\p_1}, \vec{\ell_{j}}} \Par \\ 
					& & \acc{a}{\p_m}{x} Q\lrangle{N, \srole{s}{\p_m}, \vec{\ell_{j}}}, j \in I, \p_1, \dots, \p_m \notin A.
				\end{array}
			$

		\item	$
				\begin{array}{lcl}
					Q\lrangle{N, \srole{s}{\q}, \actinp{s}{\p}{\q}{v} \cat \vec{\ell_i}} & = & 
					\out{s}{\q}{\p}{v} Q\lrangle{N, \srole{s}{\q}, \vec{\ell_{i}}} 
				\end{array}
			$

		\item	$
				\begin{array}{lcl}
					Q\lrangle{N, \srole{s}{\q}, \actbra{s}{\p}{\q}{l} \cat \vec{\ell_i}} & = &
					\sel{s}{\q}{\p}{l} Q\lrangle{N, \srole{s}{\q}, \vec{\ell_{i}}} 
				\end{array}
			$

		\item	$
				\begin{array}{lcl}
					Q\lrangle{N, a, \actreq{a}{A}{s} \cat \vec{\ell_i}} & = &
					\acc{a}{\p_1}{x} Q\lrangle{N, \srole{s}{\p_1}, \vec{\ell_{j}}} \Par \dots \Par
					\acc{a}{\p_2}{x} Q\lrangle{N, \srole{s}{\p_2}, \vec{\ell_{j}}} \Par \\
					& & \acc{a}{\p_m}{x} Q\lrangle{N, \srole{s}{\p_m}, \vec{\ell_{j}}}, j \in I, \p_1, \dots, \p_m \notin A.
				\end{array}
			$

		\item	$
				\begin{array}{lcl}
					Q\lrangle{N, \srole{s}{\q}, \actout{s}{\p}{\q}{v} \cat \vec{\ell_i}} & = &
					\inp{s}{\q}{\p}{x} \\
					& & \ifthen{x \in N}{Q\lrangle{N, \srole{s}{\q}, \vec{\ell_{i}}}} \Else\\
					& & \newsp{b}{\acc{b}{1}{x} Q\lrangle{N, \srole{s}{\q}, \vec{\ell_{i}}}}.
				\end{array}
			$

		\item	$
				\begin{array}{lcl}
					Q\lrangle{N, \srole{s}{\q}, \actdel{s}{\p}{\q}{s'}{\p'} \cat \vec{\ell_i}} & =&
					\inp{s}{\q}{\p}{x}\\
					& & \ifthen{x \in N}{Q\lrangle{N, \srole{s}{\q}, \vec{\ell_{i}}}} \Else\\
					& & \newsp{b}{\acc{b}{1}{x} Q\lrangle{N, \srole{s}{\q}, \vec{\ell_{i}}}}.
				\end{array}
			$

		\item	$
				\begin{array}{lcl}
					Q\lrangle{N, \srole{s}{\q}, \actsel{s}{\p}{\q}{l_k} \cat \vec{\ell_i}} & = &
					\bra{s}{\q}{\p}{l_k: Q\lrangle{N, \srole{s}{\q}, \vec{\ell_{i}}},\\
					& & l_i: \newsp{b}{\acc{b}{1}{x} Q\lrangle{N, \srole{s}{\q}, \vec{\ell_{i}}}}}.
				\end{array}
			$

		\item	$\begin{array}{lcl} Q\lrangle{N, n, \es} & = & R. \end{array}$
	\end{enumerate}
	
	\noi where $R = \newsp{b}{\acc{b}{1}{x} R'}$ or $R = \inact$.
	$R$ completes the session type on session channel $n$ 
	and is used to keep processes typed.

	We cannot define the test processes as a single testing
	action, which is the case in bisimulation completeness
	proofs in the untyped setting \cite{DBLP:journals/tcs/AmadioCS98,Hennessy07}.
	If that was the case then for most cases
	the parallel composition of a process
	with a single action test process would result in a
	non-typable process. For example consider process:
	$P = \out{s}{1}{2}{v} \out{s}{1}{2}{w} \inact$. If we
	choose a single action test $T = \inp{s}{2}{1}{x} \inact$ then
	the resulting parallel composition $P \Par T$ would be
	untypable.

	Instead we define tests that can test a series of actions
	and we choose the most appropriate for each process
	we want to check. Appropriate test means that
	it can test a sequence of certain actions and 
	can also yield a typable composition.

%	The tests are defined as a sequence of session actions
%	that complete the session on the testing role,
%	rather than a single action, because in the case where
%	the testing process was a single session prefix then
%	the entire testing process would be untyped with respect
%	to the global session type.

	From the definition of $T\lrangle{N, \vec{\ell_n}}$ we can show that
	$\forall T\lrangle{N, \ell \cat \vec{\ell_n}},
	T\lrangle{N, \ell \cat \vec{\ell_n}} \Trans{\ell'} T'\lrangle{N, \vec{\ell_n}}, \ell \asymp \ell'$.

	We prove the required result with induction on the
	definition of the stratified bisimilarity.

	We start with the fact that:
	\[
		\tprocess{E, \Ga}{P_1}{\De_3} \govcongs P_2 \hastype{\De_4}
	\]
	\noi Then we can $\forall \ell_{n+1} \cat \vec{\ell_n}$ we can choose
	test $T\lrangle{N, \ell_{n+1} \cat \vec{\ell_n}}$ to obtain:
	\[
		\tprocess{E, \Ga}{P_1 \Par T\lrangle{N, \ell \cat \vec{\ell_n}}}{\De_1} \govcongs
		P_2 \Par T\lrangle{N,  \ell \cat \vec{\ell_n}} \hastype{\De_2}	
	\]
	\noi If we imply that:
	\begin{eqnarray}
		\tprocess{E, \Ga}{P_1 \Par T\lrangle{N, \ell_{n+1} \cat \vec{\ell_n}}}{\De_1} &\Red&
		\noGtprocess{P_1' \Par T\lrangle{N, \vec{\ell_n}}}{\De_1'} \label{proof:cong_is_bis1}\\
		\tprocess{E, \Ga}{P_2 \Par T\lrangle{N, \ell_{n+1} \cat \vec{\ell_n}}}{\De_2} 
		&\Red&
		\noGtprocess{P_2' \Par T\lrangle{N, \vec{\ell_n}}}{\De_2'} \label{proof:cong_is_bis2}
	\end{eqnarray}
	The induction hypothesis states that:
	\begin{eqnarray*}
		\tprocess{E, \Ga}{P_1 \Par T\lrangle{N, \vec{\ell_n}}}{\De_1} &\govcongs&
		\noGtprocess{P_2 \Par T\lrangle{N, \vec{\ell_n}}}{\De_2} \textrm{ implies}\\
		\tprocess{E, \Ga}{P_1}{\De_1} &({\govwbs})_n& \noGtprocess{P_2}{\De_2}	
	\end{eqnarray*}
	So we can show from the induction hypothesis and reductions \ref{proof:cong_is_bis1} and
	\ref{proof:cong_is_bis2} that:
	\[
		\tprocess{E, \Ga}{P_1}{\De_1} ({\govwbs})_{n+1} \noGtprocess{P_2}{\De_2}	
	\]
	to obtain that $\forall n, \tprocess{E, \Ga}{P_1}{\De_1} ({\govwbs})_n \noGtprocess{P_2}{\De_2}$
	as required.
%\[
%	\begin{array}{ll}
%		& \tprocess{E, \Ga}{P_1}{\De_3} \govcongs P_2 \hastype{\De_4}\\
%		\text{Then} & \forall \ell \cat \vec{\ell_n} \textrm{ choose }
%		T\lrangle{N, \ell \cat \vec{\ell_n}}, 
%		\tprocess{E, \Ga}{P_1 \Par T\lrangle{N, \ell \cat \vec{\ell_n}}}{\De_1} \govcongs
%		P_2 \Par T\lrangle{N,  \ell \cat \vec{\ell_n}} \hastype{\De_2}\\ 
%		\Longrightarrow & 
%		\\tprocess{E, \Ga}{P_1 \Par T\lrangle{N, \ell \cat \vec{\ell_n}}}{\De_1} \Red
%		\noGtprocess{P_1' \Par T\lrangle{N, \vec{\ell_n}}}{\De_1'}, \\
%		\text{and} &\tprocess{E, \Ga}{P_2 \Par T\lrangle{N, \ell \cat \vec{\ell_n}}}{\De_2} 
%		\Red
%		\noGtprocess{P_2' \Par T\lrangle{N, \vec{\ell_n}}}{\De_2'}\\
%		\Longrightarrow &P_1' ({\govwbs})_n P_2' \quad  \textrm{(by induction hypothesis)}\\
%		\Longrightarrow &
%		\forall n, \tprocess{E, \Ga}{P_1}{\De_1} ({\govwbs})_n P_2 \hastype{\De_2}\\
%		\Longrightarrow &	\tprocess{E, \Ga}{P_1}{\De_1} \govwbs P_2 \hastype{\De_2}
%	\end{array}
%\]
	The step missing from the above syllogism requires that
	we can always find a proper test to properly reduce each process:
	\[	
		\tprocess{E, \Ga}{P_1 \Par T\lrangle{N, \ell \cat \vec{\ell_n}}}{\De_1} \govcongs
		P_2 \Par T\lrangle{N,  \ell \cat \vec{\ell_n}} \hastype{\De_2}
	\]
	\noi then
	\[
\begin{array}{ll}
&		\tprocess{E, \Ga}{P_1 \Par T\lrangle{N, \ell \cat \vec{\ell_n}}}{\De_1} \Red
		\noGtprocess{P_1' \Par T\lrangle{N, \vec{\ell_n}}}{\De_1'}\\ 
\text{and} & 
		\tprocess{E, \Ga}{P_2 \Par T\lrangle{N, \ell \cat \vec{\ell_n}}}{\De_2} \Red
		\noGtprocess{P_2' \Par T\lrangle{N, \vec{\ell_n}}}{\De_2'} 
\end{array}
	\]
We perform a case analysis on $\tprocess{E, \Ga}{P_1}{\De_3} \trans{\ell} \noGtprocess{P_1'}{\De_3'}$:\\[1mm]
{\bf Case (i):}
\[
	\begin{array}{ll}
		&\tprocess{E, \Ga}{P_1}{\De_3} \trans{\actacc{a}{A}{s}} 
		\noGtprocess{P_1}{\De_3'}\\
		\Longrightarrow 
		& \tprocess{E, \Ga}{P_1 \Par T\lrangle{N, \actacc{a}{A}{s} \cat \vec{\ell_n}}}{\De_1}\\ 		
		= & \tprocess{E, \Ga}{P_1 \Par Q\lrangle{N, a, \actacc{a}{A}{s} \cat \vec{\ell_k}} \Par
		%\dots \Par Q\lrangle{N, n, \vec{\ell_i}}}{\De_1}\\ 
		\Pi_{i\in I\setminus k} Q\lrangle{N, n, \vec{\ell_i}}}{\De_1}\\
		& \red \tprocess{E, \Ga}{P_1' \Par Q\lrangle{N, a, \vec{\ell_k}} \Par
		% \dots \Par Q\lrangle{N, n, \vec{\ell_i}}}{\De_1}\\ 
		\Pi_{i\in I\setminus k} Q\lrangle{N, n, \vec{\ell_i}}}{\De_1'}\\
		\Longrightarrow 
		& \tprocess{E, \Ga}{P_2 \Par T\lrangle{N, \actacc{a}{A}{s} \cat \vec{\ell_n}}}{\De_2}\\
		%	needs to match the reduction
		\Longrightarrow 
		& \tprocess{E, \Ga}{P_2 \Par T\lrangle{N, \actacc{a}{A}{s} \cat \vec{\ell_n}}}{\De_2} \Red
		\tprocess{E, \Ga}{P_2''' \Par T\lrangle{N, \actacc{a}{A}{s} \cat \vec{\ell_n}}}{\De_2'''}\\
		& \red
		\tprocess{E, \Ga}{P_2'' \Par T\lrangle{N, \vec{\ell_n}}}{\De_2''}
		\Red
		\tprocess{E, \Ga}{P_2' \Par T\lrangle{N, \vec{\ell_n}}}{\De_2'}
	\end{array}
\]
\noi{\bf Case (ii):}
\[
	\begin{array}{ll}
		& \tprocess{E, \Ga}{P_1}{\De_3} 
		\trans{\actinp{s}{\p}{\q}{v}} \noGtprocess{P_1}{\De_3'}\\
		\Longrightarrow
		&
		\tprocess{E, \Ga}{P_1 \Par T\lrangle{N, \actinp{s}{\p}{\q}{v} \cat \vec{\ell_n}}}{\De_1}\\
		= & \tprocess{E, \Ga}{P_1 \Par Q\lrangle{N, \srole{s}{\p}, \actinp{s}{\p}{\q}{v} \cat \vec{\ell_k}} \Par
		\Pi_{i\in I\setminus k} Q\lrangle{N, n, \vec{\ell_i}}}{\De_1}\\
		& \red
		\noGtprocess{P_1' \Par Q\lrangle{N, \srole{s}{\p}, \vec{\ell_k}} \Par
		% \dots \Par Q\lrangle{N, n, \vec{\ell_i}}}{\De_1}\\
		\Pi_{i\in I\setminus k} Q\lrangle{N, n, \vec{\ell_i}}}{\De_1'}\\
		\Longrightarrow
		&
		%\tprocess{E, \Ga}{P_2 \Par T\lrangle{N, \actinp{s}{\p}{\q}{v} \cat \vec{\ell_n}}}{\De_2}\\
		%		needs to match the reduction,
		\tprocess{E, \Ga}{P_2 \Par T\lrangle{N, \actinp{s}{\p}{\q}{v} \cat \vec{\ell_n}}}{\De_2}\\ 
		& \Red 
		\tprocess{E, \Ga}{P_2''' \Par T\lrangle{N, \actinp{s}{\p}{\q}{v} \cat \vec{\ell_n}}}{\De_2'''}\\
		&  \red
		\tprocess{E, \Ga}{P_2'' \Par T\lrangle{N, \vec{\ell_n}}}{\De_2''} \Red
		\tprocess{E, \Ga}{P_2' \Par T\lrangle{N, \vec{\ell_n}}}{\De_2'}
	\end{array}
\]
{\bf Case (iii):}
\[
	\begin{array}{ll}
		& \tprocess{E, \Ga}{P_1}{\De_3} \trans{\actout{s}{\p}{\q}{v}} 
		\noGtprocess{P_1}{\De_3'}\\
		\Longrightarrow & 
		\tprocess{E, \Ga}{P_1 \Par T\lrangle{N, \actout{s}{\p}{\q}{v} \cat \vec{\ell_n}}}{\De_1}\\
		= &		
		\tprocess{E, \Ga}{P_1 \Par Q\lrangle{N, \srole{s}{\p}, \actout{s}{p}{q}{v} \cat \vec{\ell_k}} \Par
		% \dots \Par Q\lrangle{N, n, \vec{\ell_i}}}{\De_1} \\
		\Pi_{i\in I\setminus k} Q\lrangle{N, n, \vec{\ell_i}}}{\De_1}\\
		& \Red \tprocess{E, \Ga}{P_1' \Par Q\lrangle{N, \srole{s}{\p}, \vec{\ell_k}} \Par 
		% \dots \Par Q\lrangle{N, n, \vec{\ell_i}}}{\De_1}\\
		\Pi_{i\in I\setminus k} Q\lrangle{N, n, \vec{\ell_i}}}{\De_1'}\\
		% $\tprocess{E, \Ga}{P_2 \Par T\lrangle{N, \actout{s}{\p}{\q}{v} \cat \vec{\ell_n}}}{\De_2}$
		% needs to match the reduction,
		\Longrightarrow & 
		\tprocess{E, \Ga}{P_2 \Par T\lrangle{N, \actout{s}{\p}{\q}{v} \cat \vec{\ell_n}}}{\De_2}\\
		&  \Red  
		\tprocess{E, \Ga}{P_2''' \Par T\lrangle{N, \actout{s}{\p}{\q}{v} \cat \vec{\ell_n}}}{\De_2'''}\\
		&  \Red
		\tprocess{E, \Ga}{P_2'' \Par T\lrangle{N, \vec{\ell_n}}}{\De_2''} \Red
		\tprocess{E, \Ga}{P_2' \Par T\lrangle{N, \vec{\ell_n}}}{\De_2'}
	\end{array}
\]

	The rest of the cases are similar to the above three cases.
\end{proof}
